# Supplementary material for: Composition and Resolution Dependence of Effective Coarse-Graining Potentials in Multi-Resolution Simulations
Source: arXiv:1906.01758 ancillary file (2019-06-05)
Supplement: Supplementary file 1 [file Suppl.pdf]

# **Supplementary Materials: Composition and Resolution Dependence of Effective Coarse-Graining Potentials in Multi-Resolution Simulations**

Mohammadhasan Dinpajoo and Marina G. Guenza

*Department of Chemistry and Biochemistry,*

*and Institute of Theoretical Science,*

*University of Oregon, Eugene, Oregon 97403*

(Dated: June 4, 2019)

## GENERALIZED ORNSTEIN-ZERNIKE EQUATION FOR BINARY SYSTEMS

The generalized Ornstein-Zernike (OZ) matrix relation for a binary polymeric system consisting of the monomer sites and the blob (auxiliary) sites in Fourier space is given by

$$\hat{\mathbf{H}}(k) = \hat{\mathbf{\Omega}}(k)\hat{\mathbf{C}}(k) \left[ \hat{\mathbf{\Omega}}(k) + \hat{\mathbf{H}}(k) \right], \quad (\text{S1})$$

where  $\hat{\mathbf{H}}(k)$ ,  $\hat{\mathbf{\Omega}}(k)$ , and  $\hat{\mathbf{C}}(k)$  are the total, intramolecular, and direct correlation functions for the aforementioned binary system, respectively. Each polymer is coarse-grained into a number,  $n_b$ , of blobs or CG units, and the density of blobs for a given species,  $\rho_{b\alpha}$ , is related to  $\rho_{c\alpha}$  via  $\rho_{b\alpha} = \rho_{c\alpha}n_{b\alpha}$ , where  $n_{b\alpha}$  is the number of CG units (blobs) that represent a polymer melt of type  $\alpha$ .

The correlation functions are given by

$$\hat{\mathbf{H}}(k) = \begin{bmatrix} \hat{H}_{\alpha\alpha}^{mm}(k) & \hat{H}_{\alpha\beta}^{mm}(k) & \hat{H}_{\alpha\alpha}^{mb}(k) & \hat{H}_{\alpha\beta}^{mb}(k) \\ \hat{H}_{\beta\alpha}^{mm}(k) & \hat{H}_{\beta\beta}^{mm}(k) & \hat{H}_{\beta\alpha}^{mb}(k) & \hat{H}_{\beta\beta}^{mb}(k) \\ \hat{H}_{\alpha\alpha}^{bm}(k) & \hat{H}_{\alpha\beta}^{bm}(k) & \hat{H}_{\alpha\alpha}^{bb}(k) & \hat{H}_{\alpha\beta}^{bb}(k) \\ \hat{H}_{\beta\alpha}^{bm}(k) & \hat{H}_{\beta\beta}^{bm}(k) & \hat{H}_{\beta\alpha}^{bb}(k) & \hat{H}_{\beta\beta}^{bb}(k) \end{bmatrix}, \quad (\text{S2})$$

where for a generic pair  $A, B \in (\alpha, \beta)$  we have  $\hat{H}_{AB}^{mm}(k) = \rho_{mA}\rho_{mB}\hat{h}_{AB}^{mm}(k)$ ,  $\hat{H}_{AB}^{bm}(k) = \rho_{bA}\rho_{mB}\hat{h}_{AB}^{bm}(k)$ ,  $\hat{H}_{AB}^{mb}(k) = \rho_{mA}\rho_{bB}\hat{h}_{AB}^{mb}(k)$ , and  $\hat{H}_{AB}^{bb}(k) = \rho_{bA}\rho_{bB}\hat{h}_{AB}^{bb}(k)$ .

$$\hat{\mathbf{\Omega}}(k) = \begin{bmatrix} \hat{\Omega}_{\alpha\alpha}^{mm}(k) & 0 & \hat{\Omega}_{\alpha\alpha}^{mb}(k) & 0 \\ 0 & \hat{\Omega}_{\beta\beta}^{mm}(k) & 0 & \hat{\Omega}_{\beta\beta}^{mb}(k) \\ \hat{\Omega}_{\alpha\alpha}^{bm}(k) & 0 & \hat{\Omega}_{\alpha\alpha}^{bb}(k) & 0 \\ 0 & \hat{\Omega}_{\beta\beta}^{bm}(k) & 0 & \hat{\Omega}_{\beta\beta}^{bb}(k) \end{bmatrix}, \quad (\text{S3})$$

where  $\hat{\Omega}_{\alpha\alpha}^{mm}(k) = \rho_{mA}N_A\hat{\Omega}_A^{mm}(k)\delta_{AB}$ ,  $\hat{\Omega}_{\alpha\alpha}^{mb}(k) = \rho_{bA}N_A\hat{\Omega}_A^{mb}(k)\delta_{AB}$ , and  $\hat{\Omega}_{\alpha\alpha}^{bb}(k) = \rho_{bA}n_{bA}\hat{\Omega}_A^{bb}(k)\delta_{AB}$ .

### Intramolecular Correlations: Multiblobs

Making use of the Gaussian statistics one can obtain the intramolecular form factors. The normalized monomer-monomer intramolecular form factor for a given species of  $A$ ,  $\hat{\Omega}_A^{mm}(k)$ ,

$$\hat{\Omega}_A^{mm}(k) = \frac{2}{n_{bA}^2 q_{bA}^2} (q_{bA}n_{bA} - 1 + e^{-n_{bA}q_{bA}}), \quad (\text{S4})$$

where  $q_{bA} = q_A/(n_{bA})$ ,  $q_A = k^2 < R_A^2 > /6$ , and  $R_A$  is the end to end distance of a polymer melt of type  $\alpha$  or  $\beta$ .

Treating the polymers in the CG representation as freely jointed chains, the normalized blob-monomer intramolecular form factor for a given species of  $A$ ,  $\hat{\Omega}_A^{bm}(k)$ , for multiblob models in the blob averaged limit[1] and is given by

$$\hat{\Omega}_A^{bm}(k) = \frac{1}{n_{bA}} \left[ \frac{\sqrt{\pi}}{q_{bA}^{1/2}} \text{erf} \left( \frac{q_{bA}^{1/2}}{2} \right) e^{-\frac{q_{bA}}{12}} - 2 \left( \frac{e^{-n_{bA}q_{bA}} - n_{bA}e^{-q_{bA}} + n_{bA} - 1}{n_{bA}q_{bA}(e^{-q_{bA}} - 1)} \right) e^{-q_{bA}/3} \right], \quad (\text{S5})$$

Similarly, the normalized blob-blob intramolecular form factors for a given species of  $A$ ,  $\hat{\Omega}_A^{bb}(k)$ , are given by

$$\hat{\Omega}_A^{bb}(k) = \frac{1}{n_{bA}} + 2 \left[ \frac{e^{-n_{bA}q_{bA}} - n_{bA}e^{-q_{bA}} + (n_{bA} - 1)}{n_{bA}^2(e^{-q_{bA}} - 1)^2} \right] e^{-2q_{bA}/3} \quad (\text{S6})$$

## EFFECTIVE HAMILTONIAN

The effective Hamiltonian of the polymer mixtures consisting of species represented by one or more blobs is then given by

$$H = K + U^{\text{intra}} + U^{\text{inter}}, \quad (\text{S7})$$

where  $K$ ,  $U^{\text{intra}}$ , and  $U^{\text{inter}}$  are the total kinetic, effective intramolecular, and effective inter-molecular energies. The total kinetic energy is given by

$$K = \sum_{A=1}^2 \sum_{i=1}^{n_A} \sum_{a=1}^3 \frac{p_{i a}^2}{2m_{bi a}}, \quad (\text{S8})$$

where,  $n_A$  is the number of polymers of type  $\alpha$  or  $\beta$ , and  $a = 1, 2, 3$  designates the component of the Cartesian coordinates of the  $i$ th blob with a momentum of  $p_{i a}$  and mass of  $m_{bi a}$ . Note that the blobs are treated as flexible without rigid constraints.[2]

The total effective intramolecular energy consists of the bonded and angle contributions. The total effective bonded potential is given by

$$U^{\text{bond}} = \sum_{A=1}^2 \sum_i^{n_A} \sum_{\gamma}^{n_{bA}-1} U_{\text{bond}}^{bb i \gamma}(l_{i \gamma}), \quad (\text{S9})$$

The total effective angle potential is given by

$$U^{\text{angle}} = \sum_{A=1}^2 \sum_i^{n_A} \sum_{\xi}^{n_{bA}-2} U_{\text{angle}}^{bb i \xi}(\theta_{i \xi}), \quad (\text{S10})$$

The total effective intermolecular energy is taken to be a sum of pairwise interactions and is given by

$$U^{\text{inter}} = \sum_{A,B=1}^2 \sum_i^{n_A-1} \sum_{j>i}^{n_B} \sum_{\gamma}^{n_{bA}} \sum_{\xi}^{n_{bB}} U_{AB}^{bb}(r_{ij}^{(\gamma\xi)}), \quad (\text{S11})$$

where  $\gamma$  and  $\xi$  are used to label the number of a blob along a given chain.

The classical configuration integral of the system[3, 4] may be written by

$$Z = \int \dots \int e^{-\beta(U^{\text{intra}} + U^{\text{inter}})} d\mathbf{r}, \quad (\text{S12})$$

where  $U^{\text{intra}}$  and  $U^{\text{inter}}$  are the total intramolecular and intermolecular energies and  $\beta$  is inverse temperature and  $d\mathbf{r} = \prod_{i=1}^{n_\alpha} \prod_{\gamma=1}^{n_{b\alpha}} d\mathbf{r}_i^\gamma \prod_{j=1}^{n_\beta} \prod_{\xi=1}^{n_{b\beta}} d\mathbf{r}_j^\xi$ . Therefore, the corresponding canonical partition function in this classical approximation is given by

$$Q = \frac{Z}{n_\alpha! n_\beta! \Lambda_\alpha^{(3n_\alpha \ n_{b\alpha})} \Lambda_\beta^{(3n_\beta \ n_{b\beta})}}, \quad (\text{S13})$$

where  $\Lambda_\alpha = (2\pi\beta\hbar^2/m_{b\alpha})^{1/2}$  and is the mean thermal deBroglie wavelength of a given blob for a polymer type of  $\alpha$ .

## EQUATION OF STATE

Here we provide the derivations regarding the pressure for the mixtures in the IECG formalism, where the polymers are represented by  $n_b$  coarse-grained (CG) units or blobs. The equation of state (EOS) for the mixtures consisting of  $n$  polymer chains can be obtained from the statistical mechanical definition:

$$P = k_B T \left( \frac{\partial \ln Z}{\partial V} \right)_{n,T}, \quad (\text{S14})$$

where  $P$  and  $V$  are the pressure and volume of the system and  $Z$  is the classical configuration integral of the system[3, 4] given by Eq. S12. Therefore, the pressure can be decomposed into kinetic, intramolecular, and intermolecular parts.

The kinetic contribution of the pressure for a mixture of soft spheres/multiblobs and multiblobs is obtained as

$$P_{\text{kin}} = \sum_{A=1}^2 \rho_{bA} k_B T, \quad (\text{S15})$$

where  $\rho_{bA} = \rho_{cA} n_{bA}$  and is the blob density of species  $A$  in the polymer mixture.

The intermolecular contribution of the pressure for such a mixture is then obtained as

$$P_{\text{inter}} = -\frac{2\pi}{3} \sum_{A,B=1}^2 \rho_{bA} \rho_{bB} \int_0^\infty r^3 g_{AB}^{bb}(r) \frac{\partial U_{AB}^{bb}(r)}{\partial r} dr, \quad (\text{S16})$$

where the effective CG potential,  $U_{AB}^{bb}$ , has temperature, density, degree of polymerization, and composition dependences.

In the case of multiblob models, an intramolecular contribution is added to the pressure, which consists of the harmonic part of the bond interactions,  $P_b^{\text{harm}}$ , the repulsive part of the bond interactions,  $P_b^{\text{rep}}$ , and the non-bonded interactions,  $P_{\text{nb}}$ :

$$P_{\text{intra}} = P_b^{\text{harm}} + P_b^{\text{rep}} + P_{\text{nb}}. \quad (\text{S17})$$

The pressure due to harmonic bond interactions is obtained as

$$P_b^{\text{harm}} = -\frac{4\pi}{3} \sum_A^z \rho_{cA} (n_{bA} - 1) \int_0^\infty r^3 \omega_A^{bb1}(r) \frac{\partial U_{bA}^{\text{harm}}(r)}{\partial r} dr, \quad (\text{S18})$$

where  $z$  determines the limit of summation, which  $z = 1$  for the mixture of soft spheres and multiblobs and  $z = 2$  for the mixture of two types of multiblobs. In addition,  $U_{bA}^{\text{harm}} = 9n_{bA} k_B T r^2 / (4 \langle R_A^2 \rangle)$ , and  $\omega_A^{bb1}$ , the blob-blob bond length distribution, as

$$\omega_A^{bb1}(r) = \left( \frac{3}{8\pi} \right)^{3/2} \frac{e^{-9n_{bA} r^2 / 4 \langle R_A^2 \rangle}}{(\langle R_A^2 \rangle / (6n_{bA}))^{3/2}}, \quad (\text{S19})$$

The pressure due to the repulsive part of bond interactions is obtained as

$$P_b^{\text{rep}} = -\frac{4\pi}{3} \sum_A^z \rho_{cA} (n_{bA} - 1) \int_0^\infty r^3 \omega_A^{bb1}(r) \frac{\partial U_{bA}^{\text{rep}}(r)}{\partial r} dr \quad (\text{S20})$$

with

$$U_{bA}^{\text{rep}} = U_{AA}^{bb}(r) + k_B T \ln(g_{AA}^{bb}(r)), \quad (\text{S21})$$

The pressure due to the intramolecular non-bonded interactions between the blobs, which are more than two apart is obtained as

$$P_{\text{nb}} = -\frac{4\pi}{3} \sum_A^z \rho_{cA} \int_0^\infty r^3 \omega_A^{bb>3}(r) \frac{\partial U_{AA}^{bb}(r)}{\partial r} dr \quad (\text{S22})$$

with

$$\omega_A^{bb>3}(k) = \frac{e^{-\frac{8}{3} q_{bA}} (n_{bA} - 3) + e^{-\frac{(2+3n_{bA})}{3} q_{bA}} - e^{-\frac{11}{3} q_{bA}} (n_{bA} - 2)}{(1 - e^{-q_{bA}})^2}. \quad (\text{S23})$$

## ATOMISTIC SIMULATION DETAILS

The melt of linear polyethylene chains were simulated using the TraPPE united atom force field.[5] The conventional harmonic potential was assumed to describe bond interactions (see Table S1 for details). The MD software program LAMMPS[6] was used for all simulations. All simulations were performed in canonical NVT ensemble with 3-dimensional boundary conditions, Nosé-Hoover thermostat, and standard velocity-Verlet integrator. A cutoff distance of 14 Å was used and both potential and force were required to go smoothly to zero at the cutoff distance by multiplying the potential by the Mei-Davenport-Fernando (MDF) taper function[7]

$$t(x) = \begin{cases} 1 & \text{if } r \leq r_m \\ (1-x)^3(1+3x+6x^2) & \text{if } r_m < r \leq r_c \\ 0 & \text{if } r > r_c \end{cases} \quad , \quad (\text{S24})$$

where  $r_c$  is the cutoff distance and an  $r_m$  value of 12 Å and  $x$  is given by

$$x = \frac{r - r_m}{r_c - r_m} \quad (\text{S25})$$

The united atom (atomistic) MD were performed for polymer melts with degree of polymerization,  $N$ , of 300 at a monomer density of 0.03296 sites Å<sup>-3</sup> at 503.17 K with  $N = 300$  consisting of 300 polymer chains. Although, we did not find in the literature experimental values of the pressure for this degree of polymerization, we noted that a considerable amount of experimental data at the aforementioned state points were reported for chains that were either slightly shorter or longer than our sample.[8] The data reported are compatible with the values of the pressure measured in our simulations. For all atomistic MD simulations, polymer chains were randomly generated, and overlapping chains in the initial configuration were slowly pushed apart by a soft repulsive potential. This was followed by switching on the full non-bonded potential with a small time step and performing MD simulations for an additional 1 ns while increasing the timestep to 1.25 fs. Subsequently, 200 ns were used to equilibrate and the production runs of 300 ns were performed resulting in a pressure value of  $343 \pm 4$  atm. A timestep of 2 ns was used for all production periods.

The values of the mean-square end-to-end distance measured in the atomistic simulations are found to converge during the simulation. This is important because this quantity is used

TABLE S1: TraPPE united atom force field used in this work.

| Bond potential: $U_{\text{bond}} = k_b(l - l_0)^2$                                  |                                                       |                  |
|-------------------------------------------------------------------------------------|-------------------------------------------------------|------------------|
| CH <sub>2</sub> -CH <sub>2</sub>                                                    | $k_b$ , kcal mol <sup>-1</sup> Å <sup>-2</sup>        | $l_0$ , Å        |
|                                                                                     | 450                                                   | 1.54             |
| Angle potential: $U_{\text{angle}} = k_\theta(\theta - \theta_0)^2$                 |                                                       |                  |
| CH <sub>2</sub> -CH <sub>2</sub> -CH <sub>2</sub>                                   | $k_\theta$ , kcal mol <sup>-1</sup> rad <sup>-2</sup> | $\theta_0$ , deg |
|                                                                                     | 62.1                                                  | 114              |
| Dihedral potential: $U_{\text{dih}} = \sum_i^3 \frac{C_i}{2} (1 + e_i \cos(i\phi))$ |                                                       |                  |
| CH <sub>2</sub> -CH <sub>2</sub> -CH <sub>2</sub> -CH <sub>2</sub>                  | $C_i$ , kcal mol <sup>-1</sup>                        | $e_i$            |
| $i = 1$                                                                             | 1.4110                                                | +                |
| $i = 2$                                                                             | -0.2708                                               | -                |
| $i = 3$                                                                             | 3.1430                                                | +                |
| Non-bonded potential: $U_{\text{LJ}} = 4\epsilon [(\sigma/r)^{12} - (\sigma/r)^6]$  |                                                       |                  |
| CH <sub>2</sub> -CH <sub>2</sub> -CH <sub>2</sub> -CH <sub>2</sub>                  | $\epsilon$ , kcal mol <sup>-1</sup>                   | $\sigma$ , Å     |
|                                                                                     | 0.0912                                                | 3.95             |

as an input to the IECG potential and CG simulations depend on its accuracy. The top panel of Figure S1 shows the instantaneous evolution of  $\langle R^2(t) \rangle$ . The mean-square end-to-end distance for each snapshot of the MD trajectory is defined as  $\langle R^2(t) \rangle = \sum_i^n R_i^2(t)/n$ , where  $n$  is the number polymers in the atomistic simulations. The red line in the panel shows the cumulative average; for instance at step  $j$ ,  $\langle R_j \rangle = \frac{1}{j} \sum_{i=1}^j R_i^2$ . The mean-square end-to-end distance converges during the simulation.

In addition, to monitor the structural equilibration of the polymer melts in the atomistic simulations, the average mean-square internal distances, for a given number of internal monomers  $\nu$ , were calculated in the equilibration and production periods as

$$\langle R^2(\nu) \rangle = \left\langle \frac{1}{n} \sum_{i=1}^n \left[ \frac{1}{N-\nu} \sum_{\gamma=1}^{N-\nu} (\mathbf{r}_i^\gamma - \mathbf{r}_i^{\gamma+\nu})^2 \right] \right\rangle, \quad (\text{S26})$$

where  $\nu$  is the number of monomers between the  $\gamma$ th monomer and the  $(\gamma + \nu)$ th monomer along the same chain and  $\mathbf{r}_i^\gamma$  is the position vector of monomer  $\gamma$  in chain  $i$ .

The theoretical prediction of the mean square internal distance for a freely rotating chain

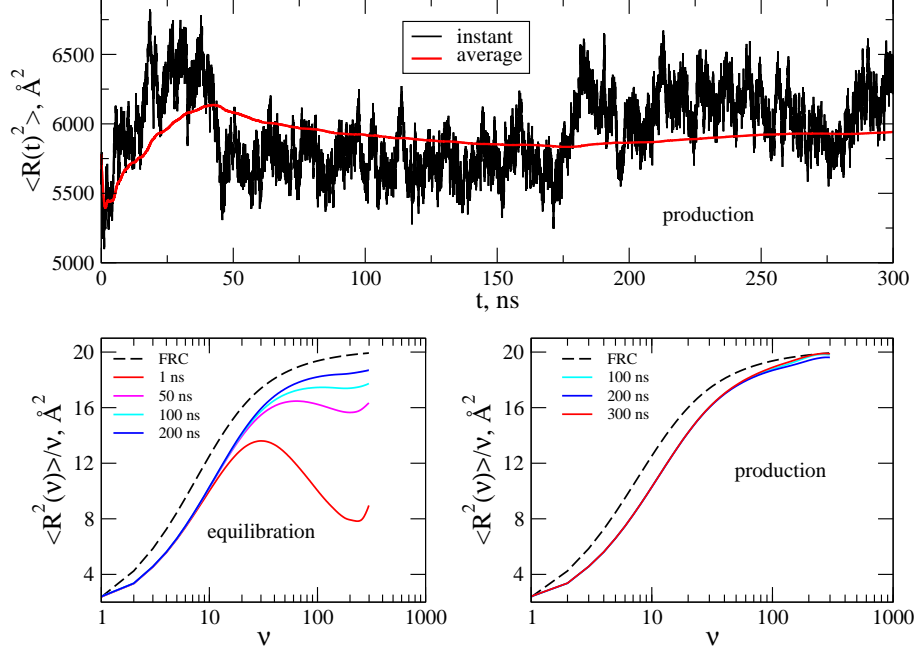

FIG. S1: Top panel: evolution of the instantaneous mean-square end-to-end distance (black line) obtained for the production period of atomistic simulations of polymers with degrees of polymerization of 300 at 503 K and a monomer density of  $0.03296 \text{ \AA}^{-3}$ . The red line shows the cumulative mean-square end-to-end distance at a given MD step. Left bottom panel: evolution of the mean-square internal distances for atomistic simulations in the equilibration period (200 ns). Right bottom panel: evolution of the mean-square internal distances for atomistic simulations in the production period (300 ns). In both bottom panels, the dashed black line shows for comparison the theoretical predictions of an idealized model for a semiflexible chains, i.e. the freely rotating chain (FRC) model.

model was calculated as

$$\langle R^2(\nu) \rangle = \nu l^2 \left[ \frac{1 - \cos \theta}{1 + \cos \theta} + \frac{2 \cos \theta}{(1 + \cos \theta)^2} \frac{1 - (-\cos \theta)^\nu}{\nu} \right], \quad (\text{S27})$$

where  $l = 1.54 \text{ \AA}$  and  $\cos \theta = -0.79$  were used to report  $\langle R^2(\nu) \rangle$  for a freely rotating chain model in Figure S1. The bottom left panel of Figure S1 compares  $\langle R^2(\nu) \rangle$  for atomistic simulations of the aforementioned system in the equilibration period. Initially, the polymers appear to be compressed due to the artifacts introduced by the preparation procedure, but the equilibration period eliminates these artifacts. The local monomer structure relaxes relatively fast due to the substantial repulsive interactions between the monomers, but the large scale chain structure require a relatively long time to equilibrate. We observed no significant change in the average mean square internal distances after 200 ns equilibration

period. The bottom right panel illustrates chain relaxation during the production period of 300 ns at every 100 ns interval: the polymer structure appears to be well equilibrated from the beginning of the production period. We also checked the rapid convergence of the pressure values (results not shown).

To investigate the temperature dependence, two additional atomistic MD simulations were performed at 463 K and 563 K. The initial configurations for these MD simulations were obtained from the last frame of the MD simulations at 503 K, and they were equilibrated for 50. Finally, 200 ns production runs were then performed at 463 and 563 K, which resulted in pressure values of  $131 \pm 3$ ,  $630 \pm 3$  atm. The square root of the average square end-to-end distance,  $\langle R^2 \rangle^{1/2}$ , from atomistic simulations was obtained as  $78.8 \pm 15.3$ ,  $76.4 \pm 16.1$ , and  $74.1 \pm 15.1$  Å at 463, 503, and 563 K, respectively, where the standard deviations were obtained from the block averages. Finally, to investigate the effect of density, atomistic simulations were also performed for polymer melts with  $N = 300$  consisting of 300 polymer chains at 503 K at two additional monomer densities of 0.03201 and 0.03429 Å<sup>-3</sup>. The initial configuration for these simulations were obtained from the final configuration of the MD simulations at a monomer density of 0.03296 Å<sup>-3</sup>. This was followed by the 20 ns equilibration MD simulations in the isobaric isothermal ensemble and 50 ns MD simulations in the canonical ensemble. The production runs for these sets of simulations consisted of 200 ns, which resulted in pressure values of  $124 \pm 4$ ,  $731 \pm 4$  atm for monomer densities of 0.03201 and 0.03429 Å<sup>-3</sup>, respectively. The values of  $\langle R^2 \rangle^{1/2}$  at monomer densities of 0.03201 and 0.03429 Å<sup>-3</sup> were found as  $77.4 \pm 14.7$  and  $76.8 \pm 14.1$  Å, respectively.

## IECG SIMULATION DETAILS

The values of  $c_{0\alpha\alpha}$  and  $\langle R_\alpha^2 \rangle$  for the IECG simulations at a given state point can be extracted from the atomistic simulations. Making use of the EOS, the  $c_{0\alpha\alpha}$  values were estimated from the pressure values of the atomistic simulations of polymer melts, e.g.  $P = 343 \pm 4$  atm for the polymer melt with  $N = 300$  at 503 K and a monomer density of 0.03296 Å<sup>-3</sup>. Therefore, the  $c_{0\alpha\alpha}$  value of  $-9.033$  Å<sup>3</sup> and  $\langle R^2 \rangle$  value of  $970$  Å<sup>2</sup>, obtained from the atomistic simulations, were used to generate the effective CG potential for all multi-resolution simulations at 503 K. The mixtures of  $n_{b4} - n_{b1}$ ,  $n_{b4} - n_{b2}$ ,  $n_{b4} - n_{b6}$ , and  $n_{b4} - n_{b10}$  were used, where  $n_{bx}$  indicates the polymer is represented by  $x$  number of blobs. The IECG

simulations allow one to directly compare the properties of such mixtures with the CG pure liquids as well as the atomistic simulations. To investigate the effect of composition, the IECG simulations for the identical polymer melts were performed at  $n_{b4}$  compositions of 0.25, 0.5, 0.75, and 1.0 at 503 and 563 K.

All IECG simulations were performed in the canonical ensemble with Nosé-Hoover thermostat and standard velocity-Verlet integrator. Periodic boundary conditions were applied in all three dimensions. Intra and inter molecular effective IECG potentials, as described in Ref. [9] were adopted, noting that in the multi-site CG (multi-blob) models the nonbonded intrachain effective CG potential involves intramolecular CG sites that are separated by more than two blobs. A cutoff distance,  $r_{\text{cut}}$ , of  $1.2\sigma_{\text{F1}}$  and appropriate neighbor skin distances were used for different mixtures, where  $\sigma_{\text{F1}}$  is the first extremum of the effective CG potential (the first zero of the force) over the range of  $r > 0$ . The combined Verlet neighbor list and the link-cell binning algorithm were used to build the Verlet neighbor list, which was updated every 10 steps.[10] A timestep of 50 fs was used for mixtures consisting of soft sphere and di-blob models. However, for six- and ten-blob simulations, a timestep of 30 fs was used. The equilibration and production periods ranged from 60-120 ns.

## THE TEMPERATURE AND DENSITY DEPENDENCES OF MULTI-RESOLUTIONS CG POTENTIALS

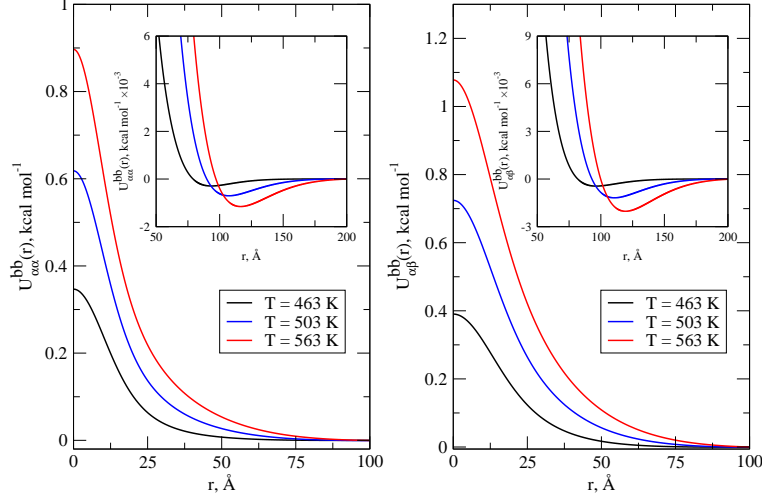

FIG. S2: The temperature dependence of the effective CG potentials between various species representing polymer melts with  $N = 300$  at various temperatures for self and cross interactions. The multi-resolution system consists of four CG units ( $\alpha$  species) and two CG units ( $\beta$  species). As the temperature increases, the range of effective CG potential for all species increases while the attractive part of the effective CG potential becomes deeper.

As discussed in the main text, the effective CG potentials are free energy. Here we discuss the temperature and density dependences for a multi-resolution system consisting of four- and di-blobs representing polymer melts with a given  $N$ .

As briefly discussed in the main text, Eqs. 10 and 12 suggest that the temperature and density dependences of the effective CG potentials can have complex behavior at various state points of the phase diagram. Figure S2 shows the temperature dependence of the effective CG potentials at a given density for all species in the mixture representing a polymer melt with  $N = 300$ . At higher temperatures the many-body effects are more pronounced, which results in longer-ranged effective CG potentials, as well as more repulsive interactions between the chains at relatively short distances.

Making use of two-particle excess entropy[11]

$$S^{(2)} \propto - \int (g_{AB}^{bb}(r) \ln g_{AB}^{bb}(r) - g_{AB}^{bb}(r) + 1) r^2 dr, \quad (\text{S28})$$

we found that the related intermolecular entropy for these polymer melts decreases as the temperature increases, which is manifested in the higher correlation hole (more ordered structure) at higher temperatures. However, at relatively large distances, the depth of the attractive part of the effective CG potential increases as the temperature increases, most likely due to the increase in the repulsive forces at short distances. Similarly, the effective CG potentials become more repulsive and long-ranged as the density increases.

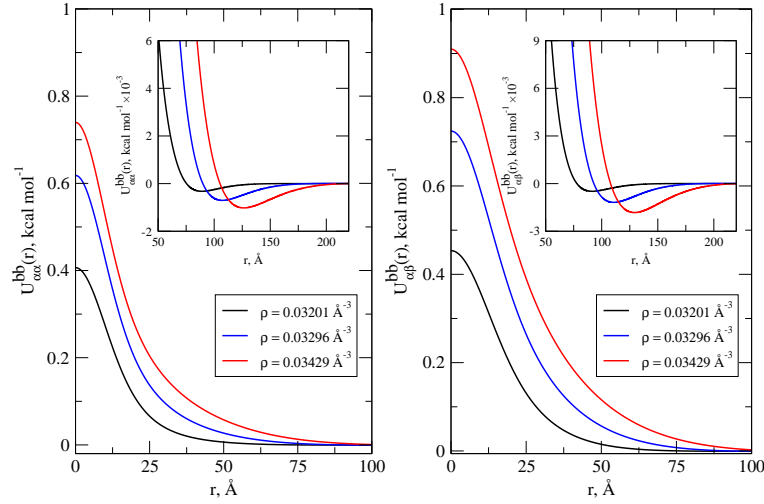

FIG. S3: The density dependence of the effective CG potentials between various species representing polymer melts with  $N = 300$  at various densities for self and cross interactions. The multi-resolution system consists of four CG units ( $\alpha$  species) and two CG units ( $\beta$  species). As the density increases, the range of effective CG potential for all species increases while the attractive part of the effective CG potential becomes deeper.

Figure S3 shows the effective CG potentials between  $n_{b4} - n_{b4}$  species as well as  $n_{b4} - n_{b2}$  species at three densities. The effective CG potentials at contact (zero separation) for all species become more repulsive as the density increases. Additionally, the range of effective CG potential increases as the density increases. Finally, the depths of the attractive parts of the effective CG potentials and the positions of their minima increase as the density increases. Therefore, both the short-range and long-range parts of the effective potential have density dependencies. Therefore, the CG procedure allows one to understand the temperature and density dependences in a rigorous way by analytical and numerical solutions.

# ANALYTICAL AND NUMERICAL MULTI-RESOLUTION CG POTENTIALS

In this Section, we compare the analytical effective CG potential obtained by the Mean-Spherical-Approximation (MSA) closure with the numerical effective CG potential obtained by the Hyper-Netted-Chain (HNC) closure. Although the second order terms are neglected in the analytical solution of the effective CG potential, Figure S4 shows that the shape and range of numerical effective CG potential are in good agreement with the analytical results.

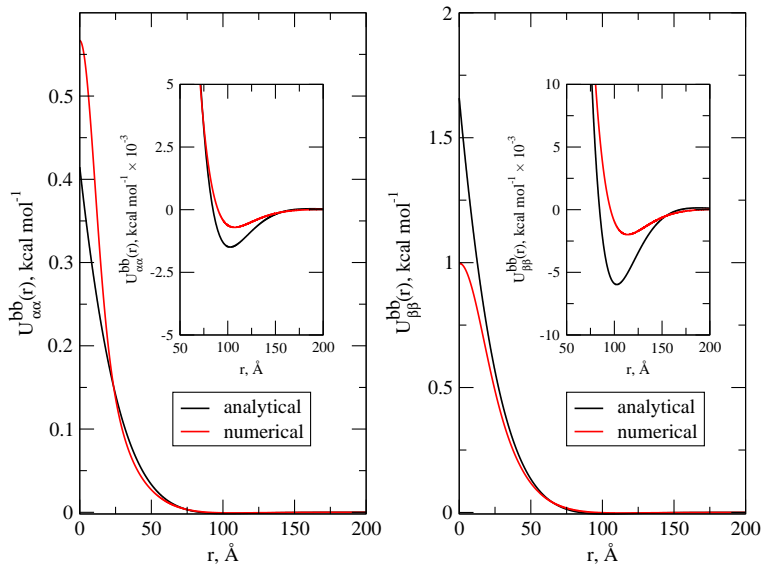

FIG. S4: Comparison of the analytical potentials by ignoring the second order terms with the numerical potentials for a multi-resolution mixture consisting of polymer melt species represented by four ( $\alpha$  species) and two ( $\beta$  species) CG units.

- 
- [1] A. J. Clark, J. McCarty, and M. G. Guenza, J. Chem. Phys. **139**, 124906 (2013).
  - [2] N. Go and H. A. Scheraga, Macromolecules **9**, 535 (1976).
  - [3] J. P. Hansen and I. R. McDonald, *Theory of Simple Liquids* (Academic Press, Amsterdam, 2003).
  - [4] K. G. Honnell, C. K. Hall, and R. Dickman, J. Chem. Phys. **87**, 664 (1987).
  - [5] M. G. Martin and J. I. Siepmann, J. Phys. Chem. B **102**, 2569 (1998).
  - [6] S. Plimpton, J. Comp. Phys. **117**, 1 (1995).
  - [7] J. Mei, J. W. Davenport, and G. W. Fernando, Phys. Rev. B. **43**, 4653 (1991).
  - [8] D. Walsh and P. Zoller, *Standard Pressure Volume Temperature Data for Polymers* (Technomic Publishing Company, Lancaster, 1995).
  - [9] M. Dinpajoo and M. G. Guenza, J. Phys. Chem. B **122**, 3426 (2018).
  - [10] M. P. Allen and D. J. Tildesley, *Computer Simulations of Liquids* (Oxford University Press, Oxford, 1987).
  - [11] A. Baranyai and D. J. Evans, Phys. Rev. A **40**, 3817 (1989).
